# Supplementary material for: Facets of the X-ray polytope of doubly stochastic matrices
Source: arXiv:2610.30058 source file (2026-10-21)
Supplement: Supplementary file 1 [file supp-labels.tex]

\makeatletter
\newlabel{sec:SM-prelim}{{SM1}{1}{}{}{}}
\newlabel{sec:SM-prelim@cref}{{[section][1][]SM1}{[1][1][]1}{}{}{}}
\newlabel{sec:SM-fan}{{SM1.1}{1}{}{}{}}
\newlabel{sec:SM-fan@cref}{{[subsection][1][1]SM1.1}{[1][1][]1}{}{}{}}
\newlabel{sec:SM-coord}{{SM1.2}{1}{}{}{}}
\newlabel{sec:SM-coord@cref}{{[subsection][2][1]SM1.2}{[1][1][]1}{}{}{}}
\newlabel{sec:SM-prelim-ex}{{SM1.3}{1}{}{}{}}
\newlabel{sec:SM-prelim-ex@cref}{{[subsection][3][1]SM1.3}{[1][1][]1}{}{}{}}
\newlabel{sec:SM-criterion}{{SM2}{2}{}{}{}}
\newlabel{sec:SM-criterion@cref}{{[section][2][]SM2}{[1][1][]2}{}{}{}}
\newlabel{sec:SM-empty}{{SM2.1}{2}{}{}{}}
\newlabel{sec:SM-empty@cref}{{[subsection][1][2]SM2.1}{[1][1][]2}{}{}{}}
\newlabel{sec:SM-symdual}{{SM2.2}{2}{}{}{}}
\newlabel{sec:SM-symdual@cref}{{[subsection][2][2]SM2.2}{[1][2][]2}{}{}{}}
\newlabel{sec:SM-fiber}{{SM2.3}{2}{}{}{}}
\newlabel{sec:SM-fiber@cref}{{[subsection][3][2]SM2.3}{[1][2][]2}{}{}{}}
\newlabel{sec:SM-cubical}{{SM3}{3}{}{}{}}
\newlabel{sec:SM-cubical@cref}{{[section][3][]SM3}{[1][3][]3}{}{}{}}
\newlabel{sec:SM-padcount}{{SM3.1}{5}{}{}{}}
\newlabel{sec:SM-padcount@cref}{{[subsection][1][3]SM3.1}{[1][5][]5}{}{}{}}
\newlabel{sec:SM-constructions}{{SM4}{5}{}{}{}}
\newlabel{sec:SM-constructions@cref}{{[section][4][]SM4}{[1][5][]5}{}{}{}}
\newlabel{sec:SM-pad}{{SM4.1}{5}{}{}{}}
\newlabel{sec:SM-pad@cref}{{[subsection][1][4]SM4.1}{[1][5][]5}{}{}{}}
\newlabel{sec:SM-refine}{{SM4.2}{6}{}{}{}}
\newlabel{sec:SM-refine@cref}{{[subsection][2][4]SM4.2}{[1][6][]6}{}{}{}}
\newlabel{sec:SM-blockgraph}{{SM4.3}{7}{}{}{}}
\newlabel{sec:SM-blockgraph@cref}{{[subsection][3][4]SM4.3}{[1][7][]7}{}{}{}}
\newlabel{sec:SM-descent}{{SM4.4}{8}{}{}{}}
\newlabel{sec:SM-descent@cref}{{[subsection][4][4]SM4.4}{[1][7][]8}{}{}{}}
\newlabel{sec:SM-famproof}{{SM4.5}{8}{}{}{}}
\newlabel{sec:SM-famproof@cref}{{[subsection][5][4]SM4.5}{[1][8][]8}{}{}{}}
\newlabel{sec:SM-fam}{{SM4.6}{9}{}{}{}}
\newlabel{sec:SM-fam@cref}{{[subsection][6][4]SM4.6}{[1][9][]9}{}{}{}}
\newlabel{sec:SM-height}{{SM4.7}{11}{}{}{}}
\newlabel{sec:SM-height@cref}{{[subsection][7][4]SM4.7}{[1][11][]11}{}{}{}}
\newlabel{sec:SM-heightZ}{{SM4.8}{11}{}{}{}}
\newlabel{sec:SM-heightZ@cref}{{[subsection][8][4]SM4.8}{[1][11][]11}{}{}{}}
\newlabel{sec:SM-divisor}{{SM4.9}{12}{}{}{}}
\newlabel{sec:SM-divisor@cref}{{[subsection][9][4]SM4.9}{[1][12][]12}{}{}{}}
\newlabel{sec:SM-steps}{{SM5}{12}{}{}{}}
\newlabel{sec:SM-steps@cref}{{[section][5][]SM5}{[1][12][]12}{}{}{}}
\newlabel{sec:SM-S}{{SM5.1}{12}{}{}{}}
\newlabel{sec:SM-S@cref}{{[subsection][1][5]SM5.1}{[1][12][]12}{}{}{}}
\newlabel{sec:SM-hingesproof}{{SM5.2}{13}{}{}{}}
\newlabel{sec:SM-hingesproof@cref}{{[subsection][2][5]SM5.2}{[1][13][]13}{}{}{}}
\newlabel{sec:SM-hinges}{{SM5.3}{13}{}{}{}}
\newlabel{sec:SM-hinges@cref}{{[subsection][3][5]SM5.3}{[1][13][]13}{}{}{}}
\newlabel{sec:SM-griddual}{{SM5.4}{14}{}{}{}}
\newlabel{sec:SM-griddual@cref}{{[subsection][4][5]SM5.4}{[1][14][]14}{}{}{}}
\newlabel{sec:SM-convminorant}{{SM5.5}{14}{}{}{}}
\newlabel{sec:SM-convminorant@cref}{{[subsection][5][5]SM5.5}{[1][14][]14}{}{}{}}
\newlabel{sec:SM-squareproof}{{SM5.6}{14}{}{}{}}
\newlabel{sec:SM-squareproof@cref}{{[subsection][6][5]SM5.6}{[1][14][]14}{}{}{}}
\newlabel{sec:SM-square}{{SM5.7}{14}{}{}{}}
\newlabel{sec:SM-square@cref}{{[subsection][7][5]SM5.7}{[1][14][]14}{}{}{}}
\newlabel{sec:SM-T3fail}{{SM5.8}{15}{}{}{}}
\newlabel{sec:SM-T3fail@cref}{{[subsection][8][5]SM5.8}{[1][14][]15}{}{}{}}
\newlabel{sec:SM-T3}{{SM5.9}{15}{}{}{}}
\newlabel{sec:SM-T3@cref}{{[subsection][9][5]SM5.9}{[1][15][]15}{}{}{}}
\newlabel{sec:SM-dec}{{SM5.10}{16}{}{}{}}
\newlabel{sec:SM-dec@cref}{{[subsection][10][5]SM5.10}{[1][16][]16}{}{}{}}
\newlabel{sec:s_census}{{SM6}{16}{}{}{}}
\newlabel{sec:s_census@cref}{{[section][6][]SM6}{[1][16][]16}{}{}{}}
\newlabel{sec:s_census-lifts}{{SM6.1}{16}{}{}{}}
\newlabel{sec:s_census-lifts@cref}{{[subsection][1][6]SM6.1}{[1][16][]16}{}{}{}}
\newlabel{tab:cores}{{SM1}{17}{}{}{}}
\newlabel{tab:cores@cref}{{[table][1][]SM1}{[1][16][]17}{}{}{}}
\newlabel{tab:shapes}{{SM2}{17}{}{}{}}
\newlabel{tab:shapes@cref}{{[table][2][]SM2}{[1][17][]17}{}{}{}}
\newlabel{sec:s_census-dict}{{SM6.2}{17}{}{}{}}
\newlabel{sec:s_census-dict@cref}{{[subsection][2][6]SM6.2}{[1][17][]17}{}{}{}}
\newlabel{sec:SM-Eflat6}{{SM6.3}{18}{}{}{}}
\newlabel{sec:SM-Eflat6@cref}{{[subsection][3][6]SM6.3}{[1][18][]18}{}{}{}}
\newlabel{sec:s_census-proofs}{{SM6.4}{19}{}{}{}}
\newlabel{sec:s_census-proofs@cref}{{[subsection][4][6]SM6.4}{[1][18][]19}{}{}{}}
\newlabel{sec:SM-S1cert}{{SM6.5}{19}{}{}{}}
\newlabel{sec:SM-S1cert@cref}{{[subsection][5][6]SM6.5}{[1][19][]19}{}{}{}}
\newlabel{app:cells}{{SM6.7}{20}{}{}{}}
\newlabel{app:cells@cref}{{[subsection][7][6]SM6.7}{[1][20][]20}{}{}{}}
\newlabel{tab:evidence}{{SM3}{21}{}{}{}}
\newlabel{tab:evidence@cref}{{[table][3][]SM3}{[1][20][]21}{}{}{}}
\newlabel{tab:cells}{{SM4}{22}{}{}{}}
\newlabel{tab:cells@cref}{{[table][4][]SM4}{[1][22][]22}{}{}{}}
\newlabel{sec:s_census-certs}{{SM6.8}{22}{}{}{}}
\newlabel{sec:s_census-certs@cref}{{[subsection][8][6]SM6.8}{[1][22][]22}{}{}{}}
\newlabel{sec:s_census-cross}{{SM6.9}{22}{}{}{}}
\newlabel{sec:s_census-cross@cref}{{[subsection][9][6]SM6.9}{[1][22][]22}{}{}{}}
\newlabel{sec:SM-walks}{{SM7}{24}{}{}{}}
\newlabel{sec:SM-walks@cref}{{[section][7][]SM7}{[1][23][]24}{}{}{}}
\newlabel{sec:SM-recursive}{{SM7.1}{24}{}{}{}}
\newlabel{sec:SM-recursive@cref}{{[subsection][1][7]SM7.1}{[1][24][]24}{}{}{}}
\newlabel{sec:SM-vertexwalk}{{SM7.2}{24}{}{}{}}
\newlabel{sec:SM-vertexwalk@cref}{{[subsection][2][7]SM7.2}{[1][24][]24}{}{}{}}
\makeatother
